# Supplementary material for: Energy-Conserving Neural Network for Turbulence Closure Modeling
Source: arXiv:2301.13770 source file (2024-03-15)
Supplement: Supplementary file 1 [file compression_exact.tex]

\section{Exact solution SGS compression for $J=2$}\label{sec:compression_exact}

For $J=2$ the minimization problem in \eqref{eq:subgrid_loss} has an exact solution.
This is obtained by equating the true local energy to the approximated local energy in the SGS variable:
\begin{equation}
\begin{split}
        \frac{1}{4}\mu_{i1}^2 + \frac{1}{4}\mu_{i2}^2 = \frac{1}{2}(\text{t}_1\mu_{i1} + \text{t}_2\mu_{i2})^2,
\end{split}
\end{equation}
assuming uniform coarse and fine grids.
Noting that $\mu_{i1}=-\mu_{i2}$ (see \eqref{eq:subgrid_zero}) we obtain $\mathbf{t}$ as
\begin{equation}
    \begin{split}
          \mu_{i1}^2=(\text{t}_1  - \text{t}_2)^2\mu_{i1}^2  \quad  \rightarrow \quad 
         1=(\text{t}_1 - \text{t}_2)^2  \quad \rightarrow \quad  \text{t}_1= \pm\frac{1}{2} + \tau_0, \quad \text{t}_2 = \mp\frac{1}{2} + \tau_0,
    \end{split}
\end{equation}
with $\tau_0 \in \mathbb{R}$. We can safely set $\tau_0$ to zero as its value does not contribute to $\text{s}_i$. This can be seen by writing the following for general $J$:
\begin{equation}
    \text{s}_i = \mathbf{t}^T\boldsymbol{\mu}_{i}=\hat{\mathbf{t}}^T\boldsymbol{\mu}_i + \cancelto{0}{\tau_0\mathbf{1}^T\boldsymbol{\mu}_i},
\end{equation}
where we decomposed $\mathbf{t}$ as variations $\hat{\mathbf{t}} \in \{\mathbf{v} \in \mathbb{R}^J:\mathbf{1}^T\mathbf{v}=0\}$ around the constant offset $\tau_0$:
\begin{equation}
    \mathbf{t} = \hat{\mathbf{t}} + \tau_0 \mathbf{1}.
\end{equation}
The relation $\mathbf{1}^T\boldsymbol{\mu}_i=0$ follows from \eqref{eq:subgrid_zero} for uniform grids.

In \ref{sec:BCs} we chose $\mathbf{t}$ such that $\mathbf{s}$ changes sign when the SGS content is reflected across the boundary, see \eqref{eq:defin_t}. Similarly, we can choose $\mathbf{t}$ as
\begin{equation}
    \mathbf{t}(\tilde{\mathbf{t}}) = (\mathbf{I} + \mathbf{P})\tilde{\mathbf{t}}
\end{equation}
ensuring that $\mathbf{s}$ is invariant, as opposed changing sign, under this reflection: 
\begin{equation*}
    \begin{split}
\text{s}_{I+i}&=\mathbf{t}^T\boldsymbol{\mu}_{I+i} = \mathbf{t}^T\mathbf{P}\boldsymbol{\mu}_{I-i+1} = \tilde{\mathbf{t}}^T(\mathbf{I}+\mathbf{P})^T\mathbf{P}\boldsymbol{\mu}_{I-i+1} =\tilde{\mathbf{t}}^T(\mathbf{I}\mathbf{P}+\underbrace{\mathbf{P}^T\mathbf{P}}_{=\mathbf{I}})\boldsymbol{\mu}_{I-i+1} \\&= \tilde{\mathbf{t}}^T(\mathbf{P}+\mathbf{I})^T\boldsymbol{\mu}_{I-i+1} = \mathbf{t}^T\boldsymbol{\mu}_{I-i+1} = \text{s}_{I-i+1},\qquad 1\leq i\leq k,
    \end{split}
\end{equation*}
for a symmetric BC applied to the right boundary.
However, this does not allow for the exact solution at $J=2$, as
\begin{equation}
    \mathbf{t}(\tilde{\mathbf{t}}) = (\mathbf{I}+\mathbf{P})\tilde{\mathbf{t}} = \left(\mathbf{I}+\begin{bmatrix}
        0 & 1 \\
        1 & 0 
    \end{bmatrix}\right)\begin{bmatrix}
        \tilde{\text{t}}_1 \\
        \tilde{\text{t}}_2 
    \end{bmatrix} = \begin{bmatrix}
        \tilde{\text{t}}_1 + \tilde{\text{t}}_2 \\
        \tilde{\text{t}}_2 + \tilde{\text{t}}_1
    \end{bmatrix}
\end{equation}
has no solutions for 
\begin{equation}
    \begin{bmatrix}
        \tilde{\text{t}}_1 + \tilde{\text{t}}_2 \\
        \tilde{\text{t}}_2 + \tilde{\text{t}}_1
    \end{bmatrix} = \begin{bmatrix}
        \pm\frac{1}{2} \\
        \mp\frac{1}{2}
    \end{bmatrix}.
\end{equation}
The choice of $\mathbf{t}$ presented in \ref{sec:BCs}, namely \eqref{eq:defin_t}, does allow for this exact solution:
\begin{equation}
    \mathbf{t}(\tilde{\mathbf{t}}) = (\mathbf{I}-\mathbf{P})\tilde{\mathbf{t}} = \left(\mathbf{I}-\begin{bmatrix}
        0 & 1 \\
        1 & 0 
    \end{bmatrix}\right)\begin{bmatrix}
        \tilde{\text{t}}_1 \\
        \tilde{\text{t}}_2 
    \end{bmatrix} = \begin{bmatrix}
        \tilde{\text{t}}_1 - \tilde{\text{t}}_2 \\
        \tilde{\text{t}}_2 - \tilde{\text{t}}_1
    \end{bmatrix} = \begin{bmatrix}
        \pm\frac{1}{2} \\
        \mp\frac{1}{2}
    \end{bmatrix} \quad \rightarrow \quad \tilde{\text{t}}_1 = \tilde{\text{t}}_2 \pm \frac{1}{2}
\end{equation}
and is therefore preferred.
